# Supplementary material for: Induction Meets Biology: Mechanisms of Repeat Detection in Protein Language Models
Source: arXiv:2602.23179 source file (2026-07-19)

Elbow Method (Inertia)

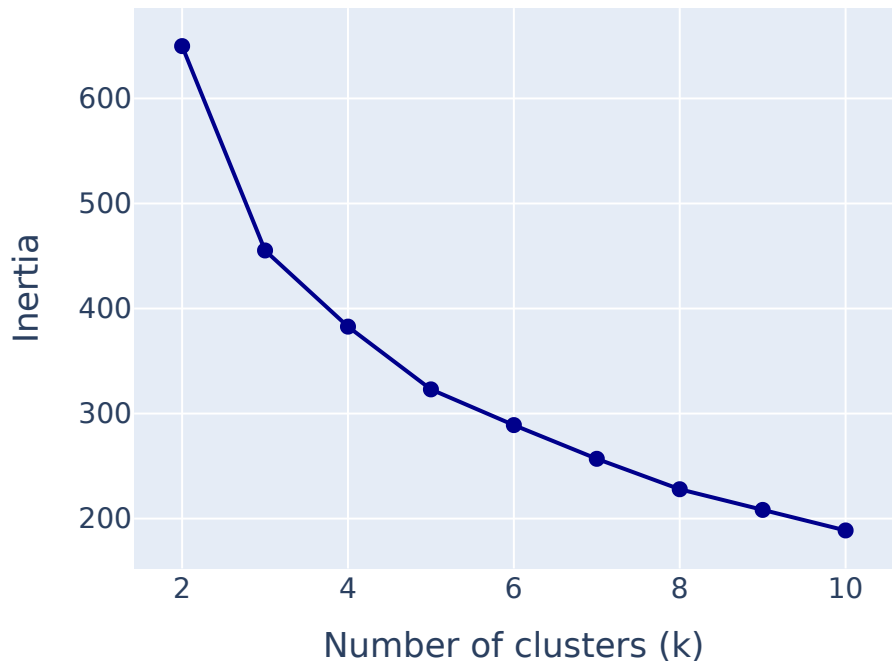

Silhouette Score

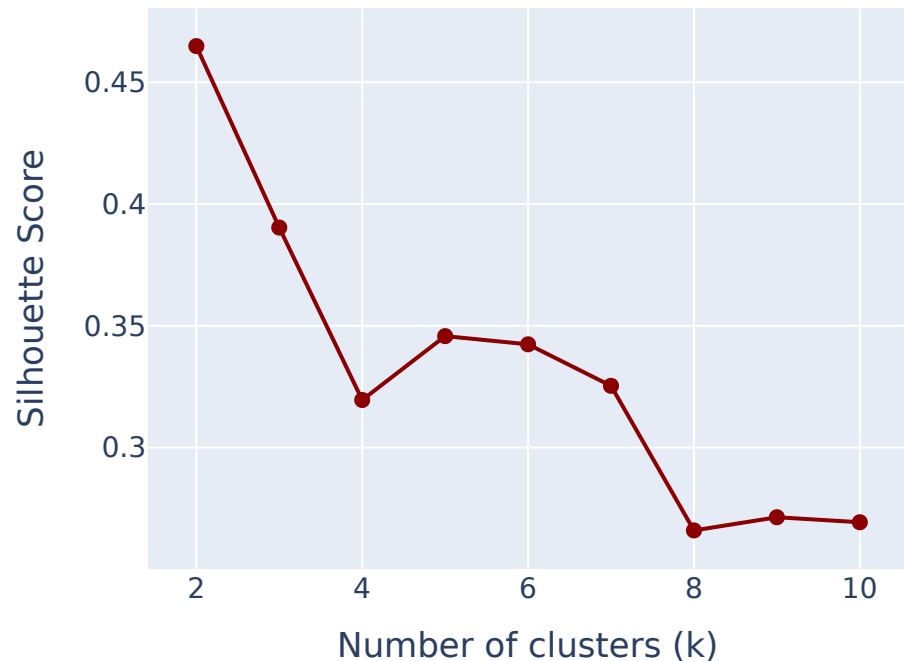

Supplement: Supplementary file 2 [file cluster_metrics_esmc.pdf]
