# Supplementary material for: Induction Meets Biology: Mechanisms of Repeat Detection in Protein Language Models
Source: arXiv:2602.23179 source file (2026-07-19)

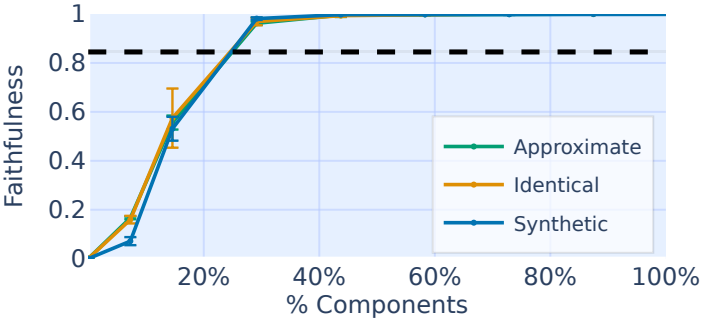

Supplement: Supplementary file 3 [file faithfulness_across_repeats_cover_all_blosum_nodes_as_first_step_for_neurons_ESMC.pdf]
