# Supplementary material for: Induction Meets Biology: Mechanisms of Repeat Detection in Protein Language Models
Source: arXiv:2602.23179 source file (2026-07-19)
Supplement: Supplementary file 4 [file neurons_esmc_sequence_visualization_m0_n2105_examples_UniRef50_A0A2K3L8W6_A0A2K3L8W6_TRIPR_MTQAGVSRIEAFQALKNNKGDIVSAIMEI.pdf]

|   |   |   |   |   |   |   |   |   |   |   |   |   |   |   |   |   |   |   |   |   |   |   |   |   |   |   |   |   |   |   |   |   |   |   |   |   |   |
|---|---|---|---|---|---|---|---|---|---|---|---|---|---|---|---|---|---|---|---|---|---|---|---|---|---|---|---|---|---|---|---|---|---|---|---|---|---|
| < | M | T | Q | A | G | V | S | K | I | E | A | V | K | A | L | T | ? | S | K | G | D | I | V | L | A | I | M | E | V | C | E | T | G | V | E | P | Y |
| D | I | D | L | V | M | T | Q | A | G | V | S | R | I | E | A | F | Q | A | L | K | N | N | K | G | D | I | V | S | A | I | M | E | I | T | S | > |   |
