# Supplementary material for: Induction Meets Biology: Mechanisms of Repeat Detection in Protein Language Models
Source: arXiv:2602.23179 source file (2026-07-19)
Supplement: Supplementary file 6 [file neurons_esmc_sequence_visualization_m20_n2224_examples_UniRef50_A0A8X6HTE9_A0A8X6HTE9_TRICU_TRKGELSRRGCSSG.pdf]

|   |   |   |   |   |   |   |   |   |   |   |   |   |   |   |   |   |   |   |   |   |   |   |   |   |   |   |   |   |   |   |   |   |   |   |   |   |   |
|---|---|---|---|---|---|---|---|---|---|---|---|---|---|---|---|---|---|---|---|---|---|---|---|---|---|---|---|---|---|---|---|---|---|---|---|---|---|
| < | M | E | T | T | R | K | G | E | L | S | R | R | G | C | S | S | G | V | E | R | S | L | R | M | R | N | V | R | G | S | N | P | P | T | A | T | L |
| T | R | F | L | R | G | H | L | L | F | L | D | T | W | T | L | P | D | W | N | G | D | T | R | K | ? | M | L | S | R | R | E | C | S | S | G | > |   |
