# Supplementary material for: Induction Meets Biology: Mechanisms of Repeat Detection in Protein Language Models
Source: arXiv:2602.23179 source file (2026-07-19)
Supplement: Supplementary file 7 [file neurons_esmc_sequence_visualization_m24_n2127_examples_MVKIWGREDGLIDRLSFFNTFDSSLRLVLYLSTIFFTVHRKFPLLKFLNSRFGHYCDFQVKFMVKIWGKKDG.pdf]

|   |   |   |   |   |   |   |   |   |   |   |   |   |   |   |   |   |   |   |   |   |   |   |   |   |   |   |   |   |   |   |   |   |   |   |   |   |
|---|---|---|---|---|---|---|---|---|---|---|---|---|---|---|---|---|---|---|---|---|---|---|---|---|---|---|---|---|---|---|---|---|---|---|---|---|
| < | M | V | K | I | W | G | R | E | D | G | L | I | D | R | L | S | F | F | N | T | F | D | S | S | L | R | L | V | L | Y | L | S | T | I | F | F |
| T | V | H | R | K | F | P | L | L | K | F | L | N | S | R | F | G | H | Y | C | D | F | Q | V | K | F | M | V | K | I | W | G | K | K | D | G | > |
