# Supplementary material for: Induction Meets Biology: Mechanisms of Repeat Detection in Protein Language Models
Source: arXiv:2602.23179 source file (2026-07-19)
Supplement: Supplementary file 10 [file neurons_esm3_sequence_visualization_m0_n125_examples_UniRef50_A0A0P7XBW1_A0A0P7XBW1_9BACT_PFFMSAARSELRSIEKTRPMGLSIP.pdf]

|   |   |   |   |   |   |   |   |   |   |   |   |   |   |   |   |   |   |   |   |   |   |   |   |   |   |   |   |   |   |   |   |   |   |   |   |   |   |
|---|---|---|---|---|---|---|---|---|---|---|---|---|---|---|---|---|---|---|---|---|---|---|---|---|---|---|---|---|---|---|---|---|---|---|---|---|---|
| < | M | S | D | T | P | F | F | M | S | A | A | R | F | E | L | R | S | M | E | K | T | R | P | ? | S | L | S | I | P | D | T | P | F | F | M | S | A |
| A | R | S | E | L | R | S | I | E | K | T | R | P | M | G | L | S | I | P | D | T | P | F | F | C | V | Y | R | T | V | W | T | Q | I | H | R | > |   |
