# Supplementary material for: Induction Meets Biology: Mechanisms of Repeat Detection in Protein Language Models
Source: arXiv:2602.23179 source file (2026-07-19)
Supplement: Supplementary file 11 [file neurons_esm3_sequence_visualization_m19_n3434_examples_UniRef50_A0A1W9X075_A0A1W9X075_9BACT_VGSIDNIRGFLSLNLGCFPRAAFF.pdf]

|   |   |   |   |   |   |   |   |   |   |   |   |   |   |   |   |   |   |   |   |   |   |   |   |   |   |   |   |   |   |   |   |   |   |   |   |   |   |
|---|---|---|---|---|---|---|---|---|---|---|---|---|---|---|---|---|---|---|---|---|---|---|---|---|---|---|---|---|---|---|---|---|---|---|---|---|---|
| < | M | R | S | G | K | W | E | V | G | S | I | D | N | I | R | G | F | L | S | L | N | L | G | C | F | P | A | L | H | F | F | Q | I | D | V | H | H |
| P | H | G | V | V | V | P | E | S | G | V | G | S | I | D | N | I | R | G | F | L | S | L | N | L | G | C | F | P | R | A | A | ? | F | S | D | > |   |
