# Supplementary material for: Induction Meets Biology: Mechanisms of Repeat Detection in Protein Language Models
Source: arXiv:2602.23179 source file (2026-07-19)
Supplement: Supplementary file 12 [file neurons_esm3_sequence_visualization_m2_n3282.pdf]

|   |   |   |   |   |   |   |   |   |   |   |   |   |   |   |   |   |   |   |   |   |   |   |   |   |   |   |   |   |   |   |   |
|---|---|---|---|---|---|---|---|---|---|---|---|---|---|---|---|---|---|---|---|---|---|---|---|---|---|---|---|---|---|---|---|
| < | M | D | S | I | Q | Y | L | R | I | P | R | T | S | S | T | K | L | F | T | K | Q | S | T | S | H | G | V | P | S | C | G |
| P | F | R | M | S | V | D | L | I | R | Y | L | H | I | P | R | T | S | S | T | ? | P | F | T | K | R | S | T | S | H | > |   |
