# Supplementary material for: Induction Meets Biology: Mechanisms of Repeat Detection in Protein Language Models
Source: arXiv:2602.23179 source file (2026-07-19)

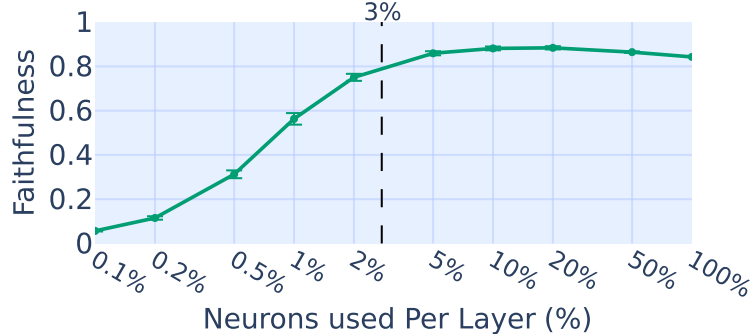

Supplement: Supplementary file 16 [file two_steps_neurons_noise_entire_repeat_cover_all_blosum_cropped.pdf]
