# Supplementary material for: Induction Meets Biology: Mechanisms of Repeat Detection in Protein Language Models
Source: arXiv:2602.23179 source file (2026-07-19)
Supplement: Supplementary file 17 [file interactions_map_esm-c.pdf]

| Src components | Input Embeddings | 1.12            | 12.14           | 5.09            | 114.27 | 0.00          |
|----------------|------------------|-----------------|-----------------|-----------------|--------|---------------|
|                | AA-biased heads  | 0.44            | 0.61            | 0.77            | 1.89   | 4.38          |
|                | Rel. Pos. heads  | 0.59            | 0.77            | 1.41            | 1.43   | 3.00          |
|                | Induction heads  | 0.48            | 1.67            | 1.94            | 6.24   | 29.89         |
|                | MLPs             | 1.22            | 1.60            | 3.57            | 6.94   | 45.84         |
|                |                  | AA-biased heads | Rel. Pos. heads | Induction heads | MLPs   | Output logits |
| Dst components |                  |                 |                 |                 |        |               |
