# Supplementary material for: Induction Meets Biology: Mechanisms of Repeat Detection in Protein Language Models
Source: arXiv:2602.23179 source file (2026-07-19)
Supplement: Supplementary file 18 [file interactions_map_esm3.pdf]

| Src components | Input Embeddings | 3.91            | 24.72           | 0.82            | 11.75 | 0.00          |
|----------------|------------------|-----------------|-----------------|-----------------|-------|---------------|
|                | AA-biased heads  | 0.25            | 0.16            | 0.85            | 1.06  | 8.52          |
|                | Rel. Pos. heads  | 0.18            | 0.24            | 1.56            | 4.18  | 2.63          |
|                | Induction heads  | 0.47            | 1.00            | 1.92            | 5.38  | 40.94         |
|                | MLPs             | 0.69            | 0.52            | 2.02            | 1.55  | 65.51         |
|                |                  | AA-biased heads | Rel. Pos. heads | Induction heads | MLPs  | Output logits |
|                |                  | Dst components  |                 |                 |       |               |
